# Supplementary material for: The Theoretical Mass--Magnitude Relation of Low-Mass Stars and its Metallicity Dependence
Source: arXiv:astro-ph/9701213 source file (1997-01-28)
Supplement: Supplementary file 1 [file appendixA.tex]

\nopagenumbers
\null

\centerline{\bf APPENDIX}

\vskip 10mm

\centerline{\null\hskip 50pt {\bf Table~A.} Derivatives of the
empirical mass-luminosity relation.}

\vskip 3mm

\hang {In the table we list our (Kroupa, Tout \& Gilmore 1993)
empirical mass--luminosity relation in bolometric magnitudes and
various photometric pass bands as a function of mass, together with
the derivatives of mass with respect to each magnitude. Masses are in
units of the solar mass. Derivatives have been multiplied by~10.
Details can be found in Section~3.2.}

\vskip 3mm

\hoffset -50pt
\hsize +540pt
$$\vbox{\tabskip=0pt \offinterlineskip
\halign to540pt{\strut#&#\tabskip=1em plus2em&
\hfil#\hfil& #&\hfil#& \hfil#& \hfil#& \hfil#& \hfil#& \hfil#&
\hfil#& \hfil#& \hfil#& \hfil#& \hfil#& \hfil#& #\tabskip=0pt\cr
& & $m$& &
$M_{\rm bol}$\hfil& $dm\over dM_{\rm bol}$\hfil& 
$M_{\rm V}$\hfil& $dm\over dM_{\rm V}$\hfil& 
$M_{\rm I}$\hfil& $dm\over dM_{\rm I}$\hfil& 
$M_{\rm J}$\hfil& $dm\over dM_{\rm J}$\hfil& 
$M_{\rm H}$\hfil& $dm\over dM_{\rm H}$\hfil& 
$M_{\rm K}$\hfil& $dm\over dM_{\rm K}$\hfil& \cr
& & & & & & & & & & & & & & & & \cr
& & 0.650 & &  7.086 & -0.993 &  8.008 & -0.725 &  6.587 & -1.050 &  5.507 & -1.420 &  4.896 & -1.480 & 4.747 & -1.610 & \cr
& & 0.635 & &  7.241 & -1.000 &  8.221 & -0.726 &  6.735 & -1.050 &  5.617 & -1.390 &  5.002 & -1.440 & 4.845 & -1.560 & \cr
& & 0.619 & &  7.395 & -1.010 &  8.434 & -0.723 &  6.882 & -1.040 &  5.731 & -1.340 &  5.112 & -1.380 & 4.946 & -1.500 & \cr
& & 0.604 & &  7.547 & -1.020 &  8.647 & -0.724 &  7.030 & -1.050 &  5.847 & -1.310 &  5.225 & -1.340 & 5.051 & -1.440 & \cr
& & 0.588 & &  7.698 & -1.030 &  8.859 & -0.731 &  7.177 & -1.060 &  5.966 & -1.290 &  5.342 & -1.310 & 5.159 & -1.410 & \cr
& & 0.573 & &  7.845 & -1.060 &  9.069 & -0.744 &  7.322 & -1.080 &  6.086 & -1.280 &  5.461 & -1.290 & 5.270 & -1.380 & \cr
& & 0.558 & &  7.988 & -1.100 &  9.273 & -0.766 &  7.463 & -1.110 &  6.206 & -1.290 &  5.580 & -1.290 & 5.382 & -1.370 & \cr
& & 0.542 & &  8.126 & -1.140 &  9.471 & -0.790 &  7.600 & -1.140 &  6.325 & -1.300 &  5.699 & -1.290 & 5.495 & -1.370 & \cr
& & 0.527 & &  8.258 & -1.190 &  9.664 & -0.812 &  7.734 & -1.170 &  6.443 & -1.320 &  5.819 & -1.300 & 5.607 & -1.370 & \cr
& & 0.511 & &  8.386 & -1.230 &  9.851 & -0.834 &  7.863 & -1.210 &  6.559 & -1.330 &  5.937 & -1.300 & 5.720 & -1.360 & \cr
& & 0.496 & &  8.509 & -1.270 & 10.034 & -0.858 &  7.990 & -1.240 &  6.675 & -1.350 &  6.056 & -1.310 & 5.834 & -1.360 & \cr
& & 0.480 & &  8.628 & -1.340 & 10.210 & -0.894 &  8.112 & -1.290 &  6.788 & -1.390 &  6.172 & -1.340 & 5.946 & -1.390 & \cr
& & 0.465 & &  8.741 & -1.400 & 10.380 & -0.928 &  8.229 & -1.340 &  6.898 & -1.420 &  6.286 & -1.370 & 6.056 & -1.410 & \cr
& & 0.450 & &  8.849 & -1.460 & 10.543 & -0.966 &  8.342 & -1.400 &  7.004 & -1.470 &  6.398 & -1.410 & 6.164 & -1.440 & \cr
& & 0.434 & &  8.952 & -1.540 & 10.699 & -1.010 &  8.450 & -1.460 &  7.107 & -1.530 &  6.505 & -1.460 & 6.269 & -1.490 & \cr
& & 0.419 & &  9.049 & -1.620 & 10.848 & -1.060 &  8.553 & -1.520 &  7.206 & -1.590 &  6.610 & -1.510 & 6.371 & -1.540 & \cr
& & 0.403 & &  9.143 & -1.690 & 10.992 & -1.100 &  8.652 & -1.580 &  7.302 & -1.650 &  6.710 & -1.560 & 6.470 & -1.590 & \cr
& & 0.388 & &  9.232 & -1.770 & 11.130 & -1.140 &  8.748 & -1.650 &  7.394 & -1.710 &  6.807 & -1.620 & 6.566 & -1.640 & \cr
& & 0.372 & &  9.317 & -1.840 & 11.263 & -1.180 &  8.840 & -1.700 &  7.482 & -1.760 &  6.901 & -1.670 & 6.658 & -1.690 & \cr
& & 0.357 & &  9.400 & -1.870 & 11.393 & -1.190 &  8.930 & -1.720 &  7.569 & -1.790 &  6.992 & -1.700 & 6.749 & -1.710 & \cr
& & 0.342 & &  9.482 & -1.890 & 11.522 & -1.200 &  9.019 & -1.730 &  7.655 & -1.810 &  7.083 & -1.710 & 6.838 & -1.730 & \cr
& & 0.326 & &  9.564 & -1.900 & 11.650 & -1.200 &  9.108 & -1.730 &  7.740 & -1.810 &  7.173 & -1.720 & 6.927 & -1.740 & \cr
& & 0.311 & &  9.645 & -1.900 & 11.779 & -1.190 &  9.197 & -1.720 &  7.825 & -1.810 &  7.263 & -1.720 & 7.016 & -1.730 & \cr
& & 0.295 & &  9.726 & -1.880 & 11.910 & -1.170 &  9.288 & -1.690 &  7.911 & -1.790 &  7.353 & -1.710 & 7.105 & -1.720 & \cr
& & 0.280 & &  9.810 & -1.800 & 12.044 & -1.110 &  9.381 & -1.610 &  7.998 & -1.710 &  7.445 & -1.630 & 7.196 & -1.650 & \cr
& & 0.264 & &  9.900 & -1.620 & 12.191 & -0.996 &  9.482 & -1.440 &  8.093 & -1.550 &  7.544 & -1.480 & 7.294 & -1.500 & \cr
& & 0.249 & & 10.001 & -1.430 & 12.356 & -0.875 &  9.596 & -1.260 &  8.198 & -1.380 &  7.654 & -1.330 & 7.402 & -1.350 & \cr
& & 0.234 & & 10.117 & -1.250 & 12.546 & -0.755 &  9.728 & -1.090 &  8.318 & -1.210 &  7.778 & -1.170 & 7.524 & -1.190 & \cr
& & 0.218 & & 10.250 & -1.070 & 12.767 & -0.644 &  9.881 & -0.931 &  8.455 & -1.050 &  7.919 & -1.020 & 7.662 & -1.050 & \cr
& & 0.203 & & 10.406 & -0.912 & 13.029 & -0.540 & 10.062 & -0.780 &  8.613 & -0.905 &  8.081 & -0.890 & 7.820 & -0.916 & \cr
& & 0.187 & & 10.587 & -0.799 & 13.337 & -0.466 & 10.275 & -0.674 &  8.794 & -0.809 &  8.264 & -0.804 & 7.997 & -0.832 & \cr
& & 0.172 & & 10.792 & -0.711 & 13.692 & -0.408 & 10.521 & -0.590 &  8.994 & -0.738 &  8.464 & -0.742 & 8.190 & -0.774 & \cr
& & 0.156 & & 11.022 & -0.636 & 14.095 & -0.358 & 10.800 & -0.517 &  9.212 & -0.680 &  8.679 & -0.692 & 8.396 & -0.727 & \cr
& & 0.141 & & 11.278 & -0.568 & 14.557 & -0.312 & 11.119 & -0.451 &  9.448 & -0.629 &  8.910 & -0.648 & 8.614 & -0.685 & \cr
& & 0.126 & & 11.567 & -0.504 & 15.088 & -0.270 & 11.487 & -0.390 &  9.703 & -0.580 &  9.156 & -0.605 & 8.846 & -0.645 & \cr
& & 0.110 & & 11.893 & -0.443 & 15.707 & -0.230 & 11.916 & -0.332 &  9.981 & -0.532 &  9.421 & -0.561 & 9.094 & -0.602 & \cr
& & 0.095 & & 12.267 & -0.383 & 16.444 & -0.191 & 12.425 & -0.275 & 10.285 & -0.481 &  9.708 & -0.512 & 9.361 & -0.553 & \cr
& & 0.079 & & 12.706 & -0.323 & 17.347 & -0.153 & 13.050 & -0.221 & 10.626 & -0.425 & 10.026 & -0.457 & 9.655 & -0.495 & \cr
}}$$

\end
